# Supplementary material for: High-Temperature Ferromagnetic Semiconductors: Janus Monolayer Vanadium Trihalides
Source: arXiv:2001.02846 source file (2020-01-14)
Supplement: Supplementary file 1 [file Supplemental-material.pdf]

Supplemental Material for

# High-Temperature Ferromagnetic Semiconductors: Janus Monolayer Vanadium Trihalides

Yulu Ren, [1] Qiaoqiao Li, [1] Wenhui Wan,[1] Yong Liu[1] and Yanfeng Ge [1, a)]

[1)]*State Key Laboratory of Metastable Materials Science and Technology & Key Laboratory for Microstructural Material Physics of Hebei Province, School of Science, Yanshan University, Qinhuangdao 066004, China*

[a)] corresponding author: **yfge@ysu.edu.cn**

## Section SI: Convergence Tests.

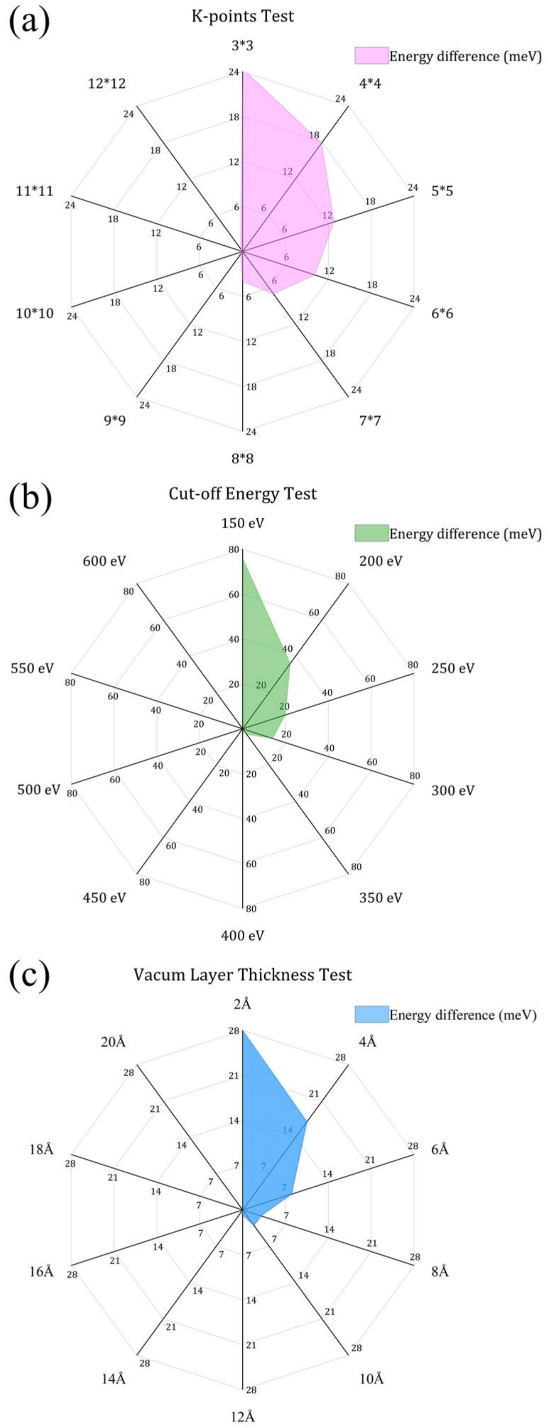


**Figure S1**. Convergence tests for a set of parameters. Energy difference ($\Delta E$) as a function of (a) number of k points, (b) cut-off energy and (c) vacuum layer thickness. Where the $\Delta E$ denotes $E - E_{12*12}$, $E - E_{600}$ and $E - E_{20Å}$ in (a), (b) and (c), respectively. The results show the three parameters reach convergence at 9*9, 450 eV and 14 Å, respectively.

## Section SII: Feasibility and Stability.

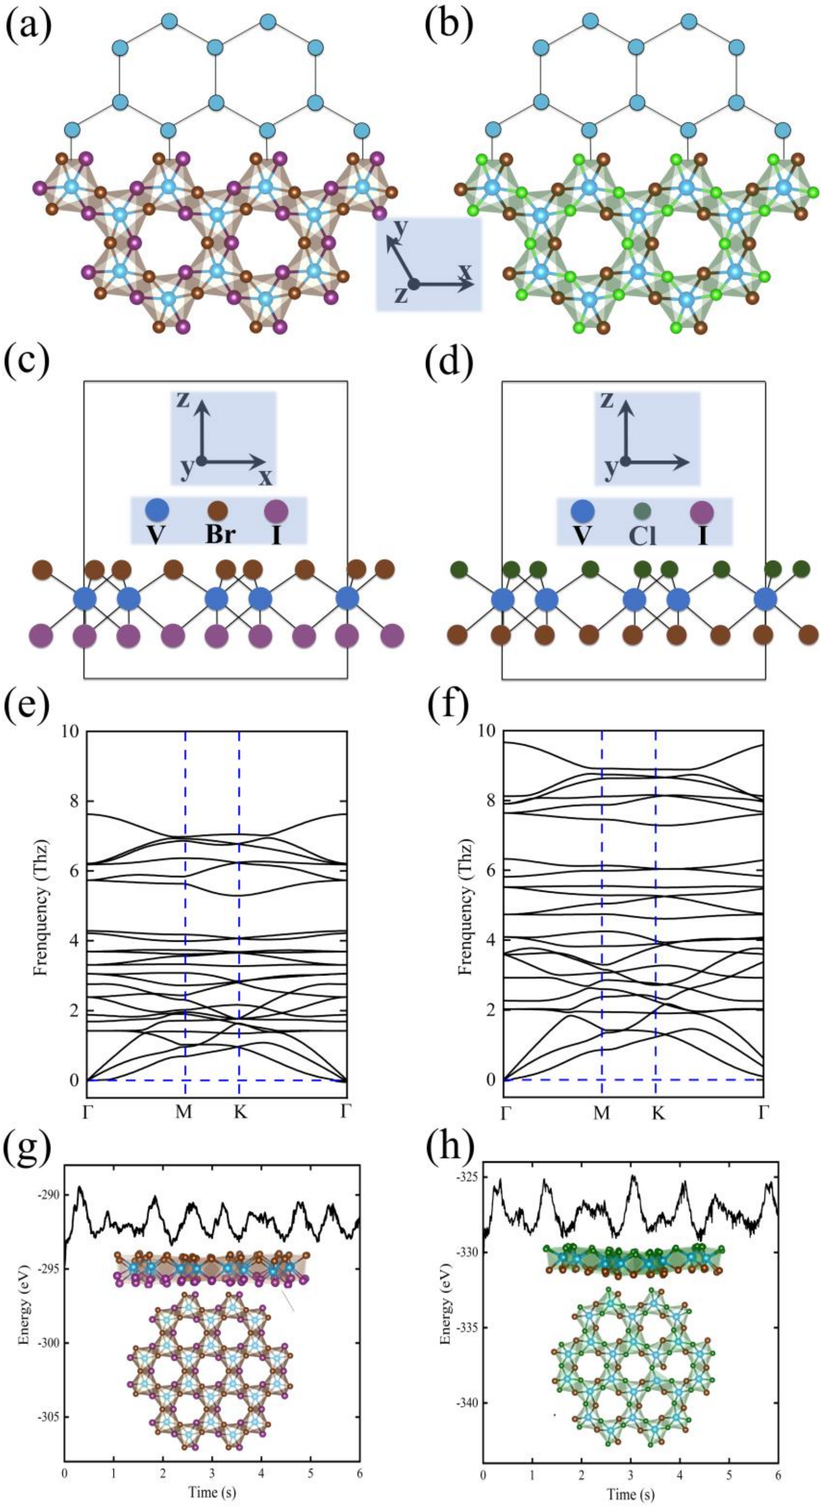


**Figure S2**. (a) Top and (c) side views of crystal structure for monolayer VBrI after full relaxation. (e) Phonon spectrum and (g) MD simulation of VBrI. (b,d,f,h) Corresponding results for monolayer VClBr.

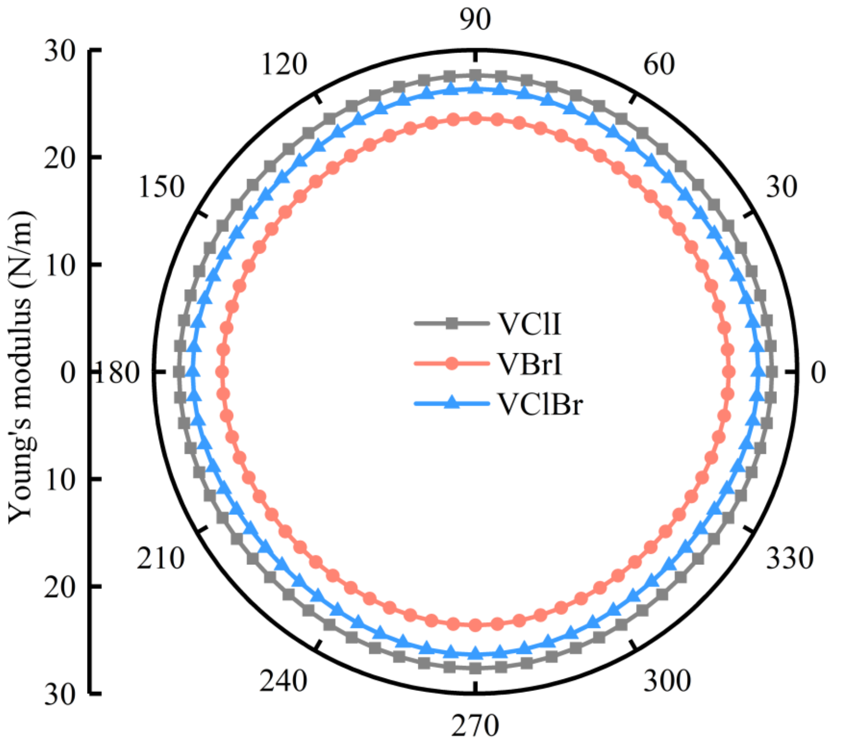


**Figure S3**. Young's module as a function of in-plane orientation, and 0° represents *a* axis. All of the three compounds show weak mechanical anisotropy character. In this work, biaxial strain is applied along *a* and *b* axis (120° angled to *a* axis). The Young's modules in the two directions are similar.

The formation energy is given by $E_f = (E_t - 3 \cdot E_X - 2 \cdot E_V - 3 \cdot E_Y)/8$, Where the $E_X$ , $E_Y$ and $E_V$ are chemical potentials of X (Y) and V atom, respectively. Taking VClI for instance, the chemical potentials are obtained from molecular crystal $Cl_2$, bcc V and solid I, respectively.

Four elastic stiffness tensors containing $C_{11}$, $C_{12}$ , $C_{22}$ and $C_{66}$ are given as follows[1]

$$C_{11} = \frac{1}{A_0} \cdot \frac{\partial^2 E_{tot}}{\partial_{\varepsilon_{11}^2}} \qquad C_{12} = \frac{1}{A_0} \cdot \frac{\partial^2 E_{tot}}{\partial_{\varepsilon_{11}} \partial_{\varepsilon_{12}}}$$

Where $A_0$ is the equilibrium area and $E_{tot}$ is total energy of the the undistorted unit cell.

Young's modulus and Poisson's rate are given as follows:

$$Y(\theta) = \frac{C_{11}C_{22} - C_{12}^2}{C_{11} \cdot sin^4\theta + A \cdot sin^2\theta cos^2\theta + C_{22} \cdot cos^4\theta}$$

$$\nu(\theta) = \frac{C_{12} \cdot sin^4\theta - B \cdot sin^2\theta cos^2\theta + C_{12} \cdot cos^4\theta}{C_{11} \cdot sin^4\theta + A \cdot sin^2\theta cos^2\theta + C_{22} \cdot cos^4\theta}$$

Where $\mathrm{A} = (C_{11}C_{12} - C_{12}^2)/C_{66} - C_{12}^2$ and $\mathrm{B} = C_{11} + C_{12} - (C_{11}C_{12} - C_{12}^2)/C_{66}$. According to the results discussed in main text, the flexible VXY monolayers can sustain a wider strain range than 2D $MoS_2$ (from -5.6% to 5.6%)[2] can do. In order to avoid wrinkles, buckle delamination and fracture effect when membranes are overstrained, a biaxial strain range from -6% to 6% is chosen in this work.

**Table SI**. The elastic constants, Young's modules and Poisson's rate of monolayer VXY. The elastic constants are determined by energy-strain approach.

| Compounds | $C_{11}$ (N/m) | $C_{22}$ (N/m) | $C_{12}$ (N/m) | $C_{66}$ (N/m) | Young's Modulus (N/m) | Poisson's Rate |
|---|---|---|---|---|---|---|
| VClI | 32.56 | 32.56 | 12.65 | 9.97 | 28.2 | 0.390 |
| VBrI | 25.93 | 25.93 | 7.68 | 8.84 | 23.7 | 0.296 |
| VClBr | 28.14 | 28.14 | 7.18 | 9.98 | 26.4 | 0.255 |

## Section SIII: Strain Induced Band Structures.

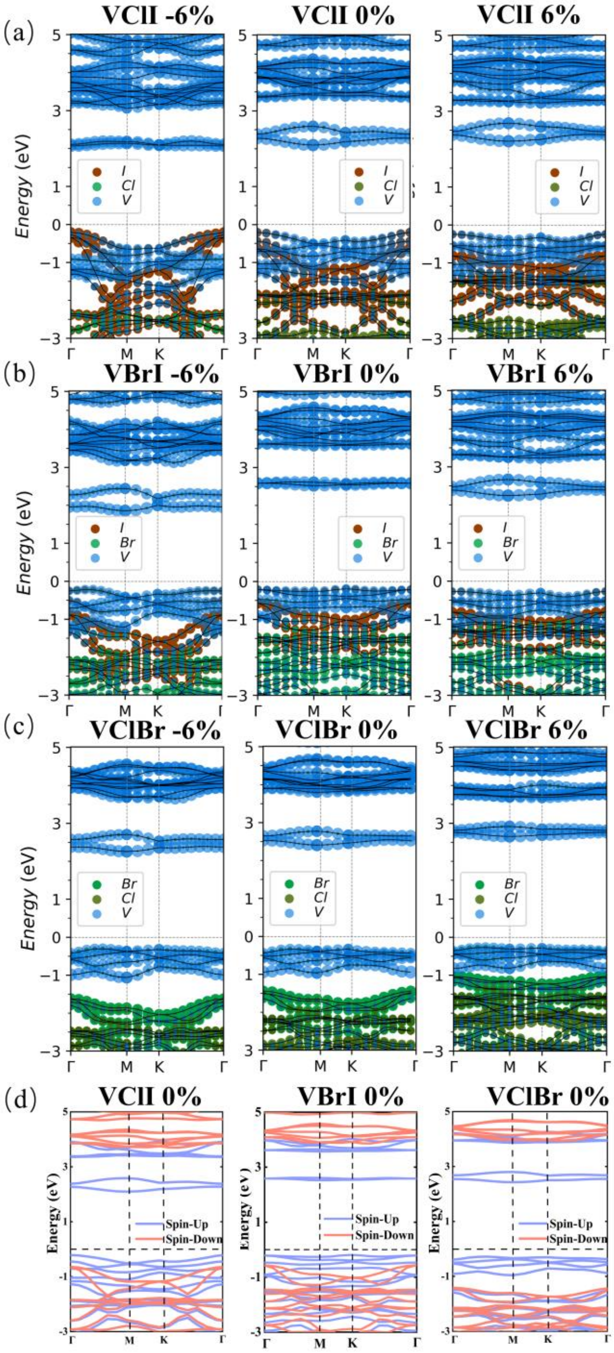

**Figure S4**. Fat band structures for monolayer VXY under biaxial strain. (a), (b) and (c) are plotted for VClI, VBrI and VClBr, respectively. The band structures are obtained by HSE06 functional. (d) Spin-polarized band structures for ground state VXY.

**Table SII**. The positions information (fractional coordinate) of valence band maximum (VBM) and conduction band minimum (CBM) in reciprocal space, as well as band gaps and main contribution under strain. According to the results, an ascendant tendency is shown in VClI and VClBr. Overall, semiconducting property remains stable and variation in gap is not large. The gaps are varied 5%, 16.3% and 18.7% in VClI, VBrI and VClBr, respectively. Then, direct band gaps are observed in monolayer VBrI and VClI but gaps for VClI are all indirect types. For band edge, the CBM is originated from V-$d$-$e_g$ while VBM is mainly contributed by $p_x$ or $p_y$ orbits of I combined with $t_{2g}$ of V in VClI and VBrI. The information in this table is obtained by HSE06 functional.

| Compounds | Strain (%) | Positions (*a*/*b*/*c*) | | Gap (eV) | Main Contribution | | Direct or indirect |
|---|---|---|---|---|---|---|---|
| | | VBM | CBM | | VBM | CBM | |
| VClI | -6 | 0/0/0 | 0.5/0.5/0 | 2.223 | I-*p* and V-*d* | V-*d* | Indirect |
| | -4 | 0/0/0 | 0/0.5/0 | 2.249 | I-*p* and V-*d* | V-*d* | Indirect |
| | -2 | 0/0/0 | 0/0.5/0 | 2.270 | I-*p* and V-*d* | V-*d* | Indirect |
| | 0 | 0/0/0 | 0.5/0/0 | 2.302 | I-*p* and V-*d* | V-*d* | Indirect |
| | 2 | 0.75/0.25/0 | 0.5/0.5/0 | 2.348 | I-*p* and V-*d* | V-*d* | Indirect |
| | 4 | 0.75/0.25/0 | 0.5/0.5/0 | 2.360 | I-*p* and V-*d* | V-*d* | Indirect |
| | 5 | 0.75/0.25/0 | 0.5/0.5/0 | 2.383 | I-*p* and V-*d* | V-*d* | Indirect |
| VBrI | -6 | 0.3/0.3/0 | 0.5/0.5/0 | 2.383 | I-*p* and V-*d* | V-*d* | Indirect |
| | -4 | 0.08/0/0 | 0/0/0 | 2.353 | I-*p* and V-*d* | V-*d* | Indirect |
| | -2 | 0.08/0/0 | 0.5/0.5/0 | 2.482 | I-*p* and V-*d* | V-*d* | Indirect |
| | 0 | 0.3/0.3/0 | 0/0.5/0 | 2.716 | I-*p* and V-*d* | V-*d* | Indirect |
| | 2 | 0.5/0.5/0 | 0.5/0.5/0 | 2.336 | I-*p* and V-*d* | V-*d* | Direct |
| | 4 | 0.5/0.5/0 | 0.5/0.5/0 | 2.351 | I-*p* and V-*d* | V-*d* | Direct |
| | 5 | 0.5/0.5/0 | 0.5/0.5/0 | 2.402 | I-*p* and V-*d* | V-*d* | Direct |
| VClBr | -6 | 0.6/0.4/0 | 0.5/0/0 | 2.422 | V-*d* | V-*d* | Indirect |
| | -4 | 0.6/0.4/0 | 0.5/0/0 | 2.476 | V-*d* | V-*d* | Indirect |
| | -2 | 0.6/0.4/0 | 0.5/0/0 | 2.537 | V-*d* | V-*d* | Indirect |
| | 0 | 0.6/0.4/0 | 0.5/0/0 | 2.645 | V-*d* | V-*d* | Indirect |
| | 2 | 0.5/0.5/0 | 0.5/0.5/0 | 2.658 | V-*d* | V-*d* | Direct |
| | 4 | 0.6/0.4/0 | 0.5/0/0 | 2.813 | V-*d* | V-*d* | Indirect |
| | 5 | 0.6/0.4/0 | 0.5/0/0 | 2.876 | V-*d* | V-*d* | Indirect |

## Section SIV: Estimations of $G_{ex}$ between $t_{2g}$ and $e_g$ of nearest-neighbor transition metal atoms.

We have discussed in main text the virtual exchange gap between $e_g$ and $t_{2g}$ states is 2.156 eV in $CrI_3$, larger than 1.732 eV in VClI. These values are obtained by estimating the on-site energies of *d* orbits of each transition metal atom based on maximally localized Wannier functions (MLWFs) obtained with the Wannier90 package. The Cr-*d* and I-*p* orbits are adopted as projections to construct WFs for monolayer $CrI_3$, V-*d* and I-*p* for $VI_3$, V-*d*, X-*p* and Y-*p* for VXY. An appropriate inner and outer energy windows are used during the disentanglement procedure. We find in each transition atom, three Hamiltonian matrix elements $\langle 0n|H|0n\rangle$ values are resembled (the difference is less than 1%) which denote triple degenerated $t_{2g}$ level stagger while two Hamiltonian matrix elements are resembled which denote double degenerated $e_g$ level stagger. Theoretically, two V atoms in a primitive cell of monolayer $VX_3$ are equivalent, so the splitting energies $\Delta c$ for *d* orbits should be the same and are equal to $G_{ex}$. In fact, that is not the case, the crystal-field splitting energies in two V atoms in a unit cell are different although the periodical lattice is fully relaxed. As a consequence, different $G_{ex}$ values occur in one figure and the larger one is used.

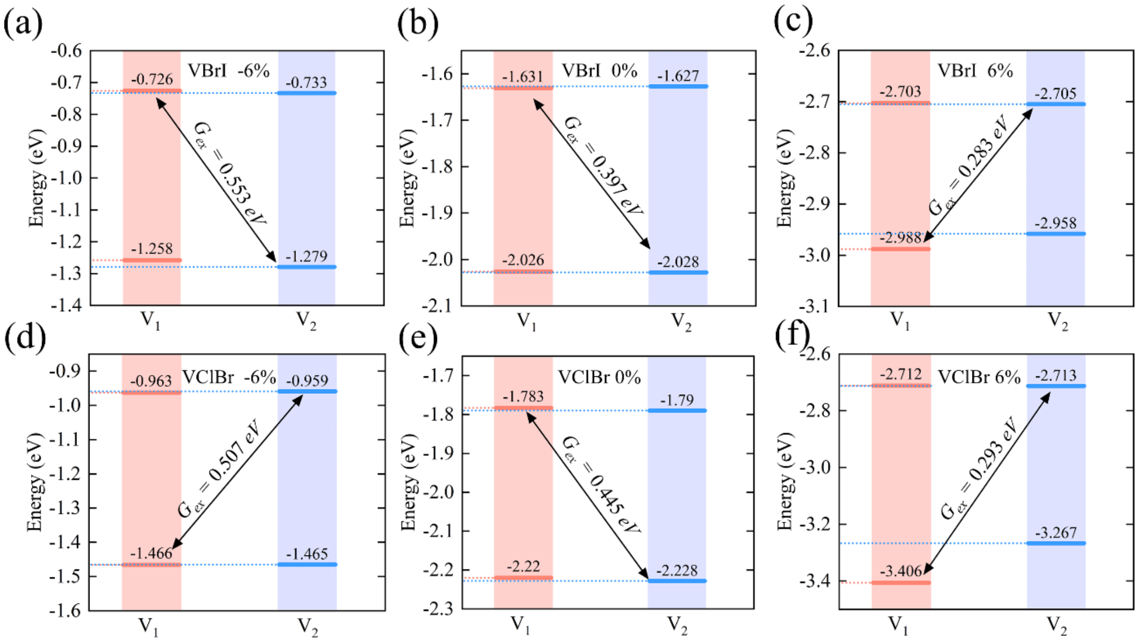


**Figure S5**. On-site energies for $e_g$ and $t_{2g}$ level staggers of monolayer (a-c) VBrI and (d-f) VClBr under biaxial strain.

## Section SV: Electronic Properties.

Figure 4c in the main text and Figure S9 in supplement material are obtained based on lobster code. Taking VClI for instance, we use V-3*d*4*s*, Cl-3*s*3*p* and I-5*s*5*p* to build the basic functions. PbeVaspFit2015 is employed based on koga but with additional functions fitted by S. Maintz to atomic VASP GGA-PBE wavefunctions. Abs. chg. spl. in inset of Figure 4c in main text means average of spilling over occupied bands. The smaller the value is, the more reasonable the basic functions and results are. Typically, the charge spilling under 5% could be considered good.

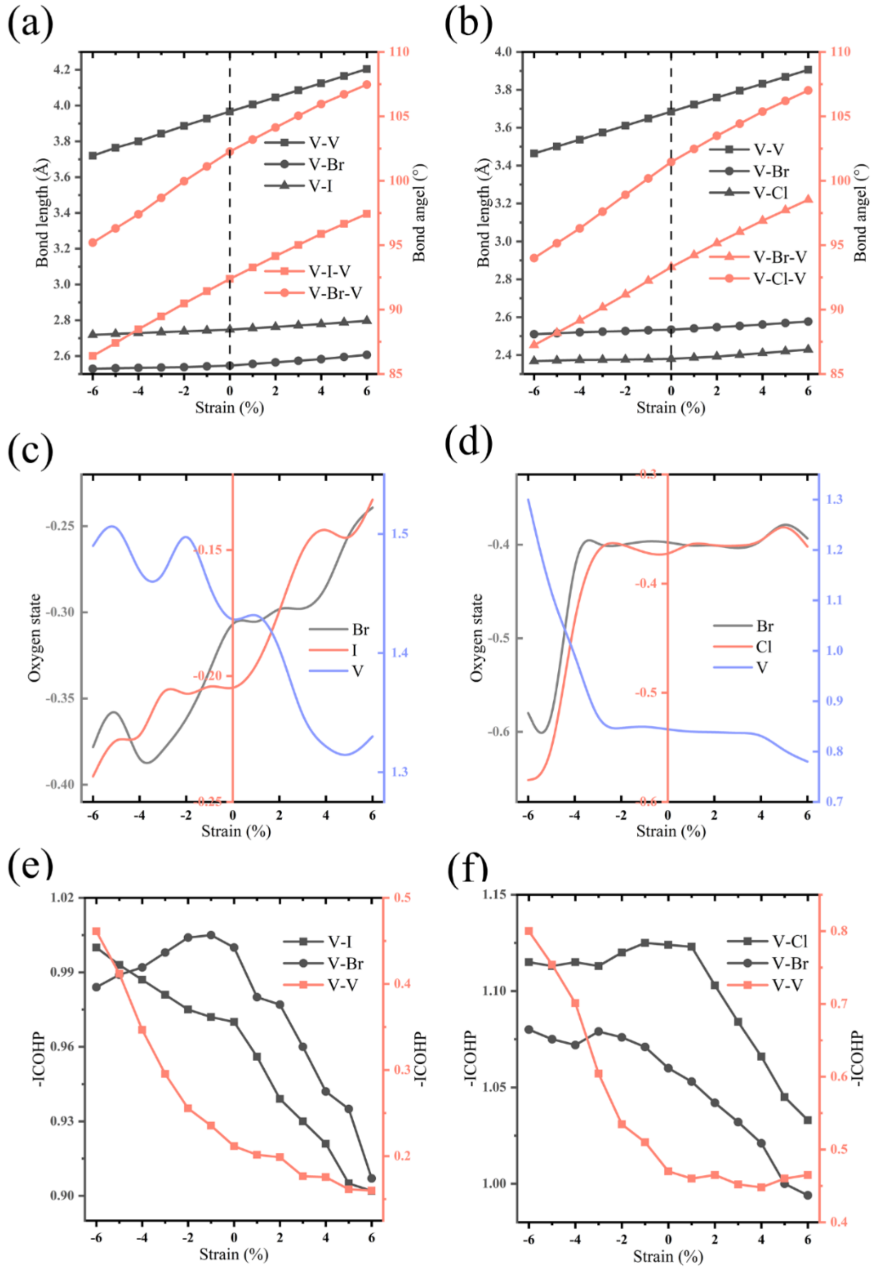


**Figure S6**. (a) Bond lengths as well as (b) bond angels of monolayer VBrI and VClBr, as the function of biaxial strain. The average oxygen states for a unit cell of monolayer (c) VBrI and (d) VClBr based on Bader charge analysis with HSE06 functional. The average opposite ICOHP values for monolayer (e) VBrI and (f) VClBr based on crystal orbital Hamilton population analysis (COHP).

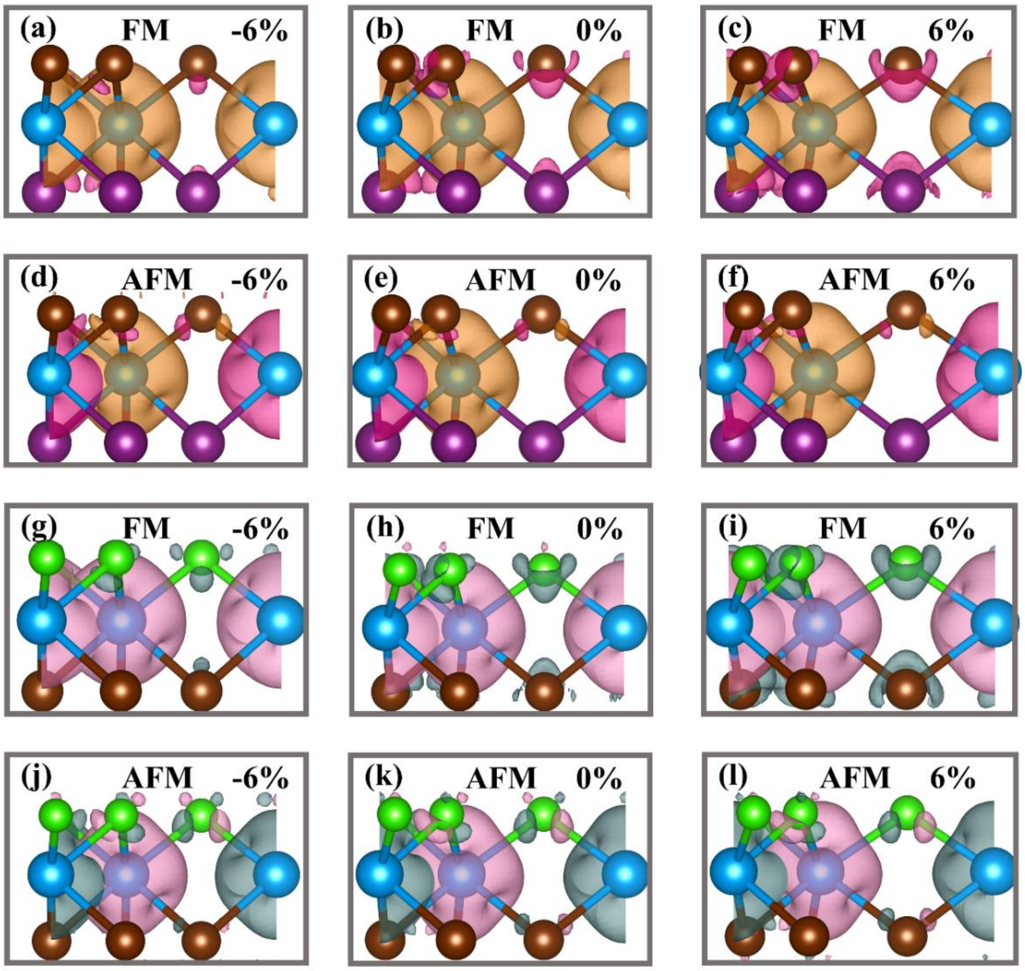


**Figure S7**. Spin density for AFM and FM of monolayer VBrI and VClBr under different strain. (a-f) Orange and pink denote majority and minority spin channels, respectively. (g-l) Pink and gray denote majority and minority spin channels, respectively. The isosurface values of all panels are set to 0.0031 eV/Å$^3$. The spin density diagrams are obtained based on HSE06 functional. Spin density for FM (AFM) increases (decreases) with the increasing lattice parameters. Therefore, the tendencies for VBrI and VClBr are consistent with VClI in the main text.

**Table SIII**. Mulliken, Löewdin and Bader charge analyses for VXY. The three kinds of charge, determined based on HSE06 functional.

| Compounds | Atoms | Mulliken charge | Löewdin charge | Bader charge |
|---|---|---|---|---|
| VClI | I | -0.51 | -0.43 | -0.48 |
| | Cl | -0.57 | -0.44 | -0.69 |
| | V | 1.63 | 1.40 | 1.76 |
| VBrI | I | -0.50 | -0.43 | -0.50 |
| | Br | -0.55 | -0.48 | -0.67 |
| | V | 1.61 | 1.42 | 1.72 |
| VClBr | Br | -0.55 | -0.47 | -0.55 |
| | Cl | -0.56 | -0.48 | -0.61 |
| | V | 1.68 | 1.43 | 1.81 |

## Section SVI: Magnetic Phase.

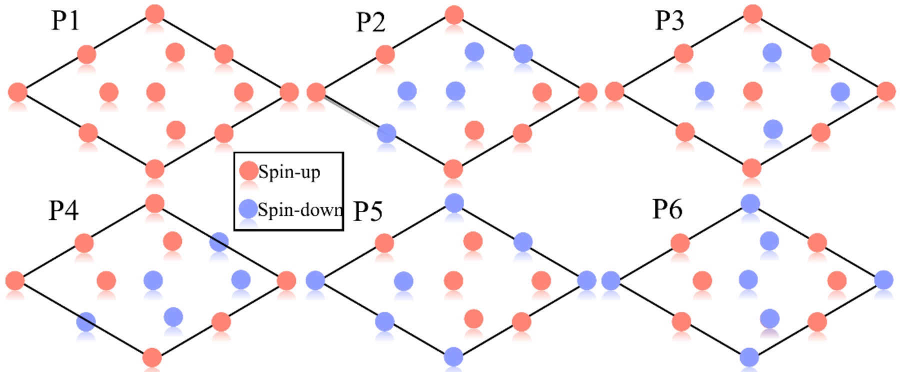


**Figure S8**. Six kinds of spin configurations of monolayer VXY, where P1, P2, P3 and P4 represent FM, Zigzag, Neél and Stripy spin arrays, respectively. Each crystal plotted above is schematic diagram of a $2 \times 2$ supercell and only V atoms are shown.

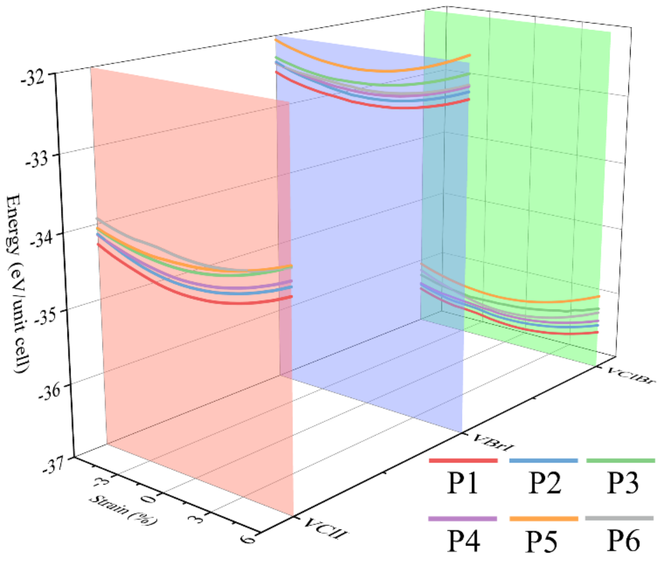


**Figure S9.** System energy per unit cell of monolayer VClI, VBrI and VClBr, as a function of biaxial strain. Six spin arrays are plotted in this figure. The results show FM are ground state in the three compounds and the Zigzag arrays are most stable between AFM spin arrays.

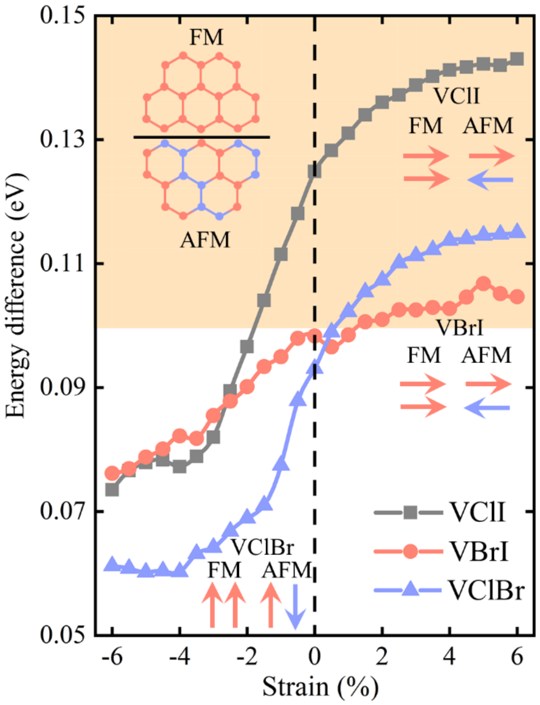


**Figure S10**. Energy difference between FM and AFM per unit cell as a function of biaxial strain and the inset shows FM and Zigzag-AFM arrays used to calculate. So, positive values represent FM ground state while negative values represent AFM ground state.

## Section SVII: Monte Carlo simulations of Curie temperature via Heisenberg and Ising model:

In this part we estimate the Curie temperature ($T_C$) for monolayer VXY. The estimating approach is based on the fact that quantum effects tend to be quenched by thermal fluctuations and one can consider a classical approximation for the model. The $T_C$ can then be obtained of the model at different temperature and find the point where the average magnetism vanishes. Firstly, we discuss Monte Carlo simulation by Ising model. The model Hamiltonian is considered as follows:[3]

$$\hat{H} = -\sum_{ij} J_{ij}\, \boldsymbol{S}_i \cdot \boldsymbol{S}_j$$

where the summation i runs over all nearest-neighbor pairs and j runs over the six nearest neighbors of site i. $J_{ij}$ is the nearest-neighbor exchange parameter. Only consider the nearest correlation, the exchange coupling constant $J$ is given by:

$$E_{ex} = -2zJS^2 \quad (2)$$

Where the $E_{ex}$ is the energy difference between equilibrium AFM and FM states and $z$ is the number of the nearest magnetic atoms. In hexagonal honeycomb system $z$ = 3. Then, $S$ = 1, which is consistent with the magnetic moment of $2\mu_B$ each V atom. According to the result, equilibrium-state $T_C$ of monolayer VClI, VBrI and VClBr are evaluated as 357, 270 and 259 K, respectively. We find Ising model simulations do in general yield agreement with experiments in Cr-based monolayer and bulk materials but large deviations occur in V-based and other S ≤ 1 systems (generally, much larger than experimental values). The estimated $T_C$ for monolayer $VI_3$ with Ising model is 223 K while the experimental value is 50 K. We consider the reasons for the overestimation in monolayer

V-based trihalides are completely failing to take into consideration the single-site magnetic anisotropy which is a crucial factor for ferromagnetic transition-metal trihalides.[4] Additionally, the directions for spins in Ising model are only vertical to ab-plane, not consistent with our results. Therefore, large deviated values occur in V-based trihalides.

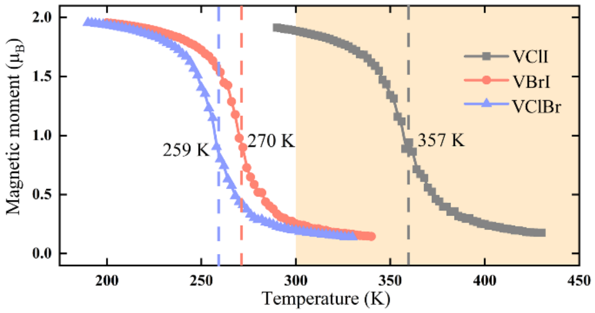


**Figure S11**. Magnetic moment of ground state monolayer VXY with respected to temperature obtained from Ising-model-MC simulations. Additionally, orange denotes the area above room temperature.

For an accurate estimation of Curie temperature, we then apply Heisenberg model. The Hamiltonian is given as follows:[5,6]

$$\hat{H} = -\sum_{ij} J_{ij}\,\boldsymbol{S}_i \cdot \boldsymbol{S}_j - A\sum_{i} (S_i^z)^2$$

with $J_{ij}$, A > 0 and A is the single-site magnetic anisotropy parameter. The detail of the Metropolis algorithm can be found in the reference[7]. Herein, we only emphasize the method of choosing random $\theta$,$\varphi$ (this can be found in reference[7] pp. 399). In order to generate our random, spherically symmetric unit vectors, we should choose:

$$\theta = \cos^{-1}(1-2r_1)$$

$$\varphi = r_2 \cdot 2\pi$$

Where $r$ is the random number between 0 to 1.

The following is the detail for computing $J_1$, $J_2$, and $J_3$ and we have the following energies for monolayer VXY with the FM order and the P2, P3 and P4 orders (Figure S8).

$$E_{P1} = E_0 + (3J_1 + 6J_2 + 3J_3)S^2$$

$$E_{P2} = E_0 + (J_1 - 2J_2 - 3J_3)S^2$$

$$E_{P3} = E_0 + (-3J_1 + 6J_2 - 3J_3)S^2$$

$$E_{P4} = E_0 + (-J_1 - 2J_2 + 3J_3)S^2$$

Where, $E_0$ is the energy of the spin-nonpolarzied configuration.

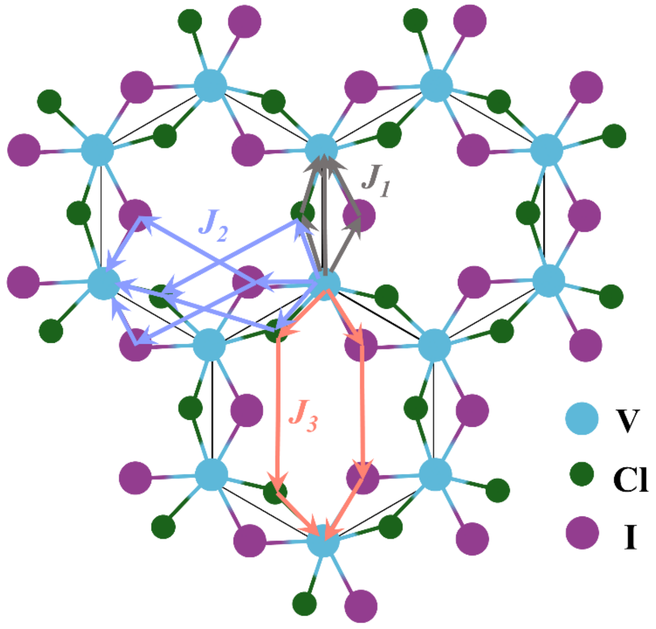


**Figure S12**. Top view of monolayer VClI, the blue, green and purple denote V, Cl and I atoms, respectively. $J_1$, $J_2$ and $J_3$ are the nearest-neighbor (NN), 2nd-NN and 3rd-NN coupling constants, respectively. Actually, there are plenty of exchanging paths between two V atoms which are not shown and only the most favorable paths are displayed in this figure.

**Table SIV**. Exchange coupling constants $J_1$, $J_2$ (the 2nd-NN), $J_3$ (the 3rd-NN), single-ion magnetic anisotropic energy (MAE) and Curie temperature under biaxial strain.

| Compounds | Strain (%) | $J_1$ (meV) | $J_2$ (meV) | $J_3$ (meV) | MAE (meV) | *Tc* (K) |
|---|---|---|---|---|---|---|
| $VI_3$ | 0 | 22.5 | 6.27 | 9.15 | 0.6 | 96 |
| VClI | -6 | 24.5 | 3.25 | 9.8 | -0.4 | 132 |
| | 0 | 48.26 | -2.26 | 5.41 | -0.6 | 240 |
| | 6 | 52.7 | -6.2 | 5.9 | -0.7 | 280 |
| VBrI | -6 | 23.6 | 3.8 | 10.4 | -1.2 | 120 |
| | 0 | 41.25 | -3.75 | 3.75 | -1.1 | 224 |
| | 6 | 49.76 | -4.13 | 4.9 | -1.4 | 272 |
| VClBr | -6 | 24.5 | 3.3 | 9.8 | 0.2 | 136 |
| | 0 | 46.7 | -5.4 | 4.9 | 0.3 | 232 |
| | 6 | 54.5 | -5.1 | 6.5 | 0.1 | 277 |

**Table SV**. The calculated and reference values of lattice parameters $a$ and Curie temperature $T_C$. The boldfaces denote experimental values. The compounds chosen to estimate are all with similar hexagonal honeycomb structure. Among these compounds, one magnetic atom is combined with six halogen atoms forming octahedral symmetry. This table shows the estimated $T_C$ yield much agreement with experimental values.

| Compounds | Estimated $a$ (Å) | Ref. values of $a$ (Å) | Estimated $Tc$ (K) | Ref. values of $T_C$ (K) | Ref. |
|---|---|---|---|---|---|
| $CrI_3$ | 6.907 | **6.87**, 7.00 | 37 | **45** | [8–11] |
| $CrBr_3$ | 6.446 | 6.44. 6.43 | 50 | 41, **47** (bulk) | [8–10] |
| $CrCl_3$ | 6.070 | 6.06, 6.05 | 22 | 30, **27** (bulk) | [8–10] |
| $CrGeTe_3$ | 6.813 | 6.86 **6.82** | 78 | **67.9** | [12] |
| $CrSiTe_3$ | 6.768 | 6.78 **6.76** | 53 | **32.9** | [13] |
| $VI_3$ | 6.824 | **6.83** | 96 | **51, 50** (bulk) | [14–16] |
| VClI | 6.62 | ---- | 240 | ---- | ---- |
| VBrI | 6.79 | ---- | 224 | ---- | ---- |
| VClBr | 6.30 | ---- | 232 | ---- | ---- |

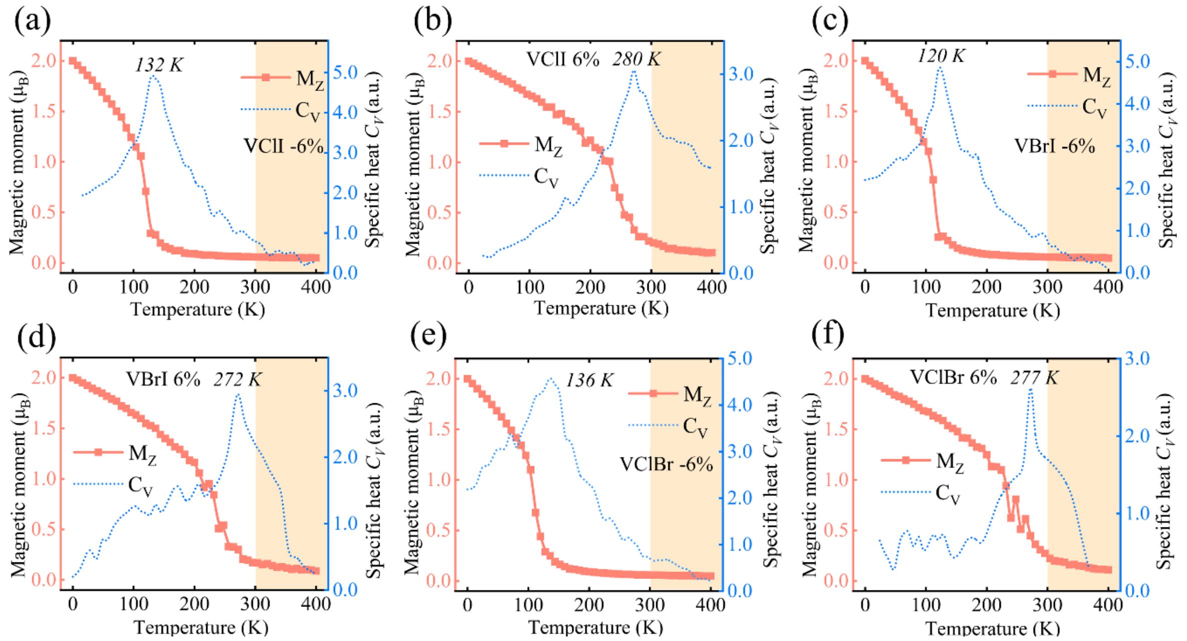


**Figure S13**. Magnetic moment per V ion and specific heat $C_V$ per unit cell as a function of temperature, (a-b) for monolayer VClI, (c-d) for VBrI and (e-f) for VClBr under strain of -6% and 6%, respectively. Orange denotes the areas above room temperature.

## Section SVIII: References


(1) Cadelano, E.; Palla, P. L.; Giordano, S.; Colombo, L. Elastic Properties of Hydrogenated Graphene. *Phys. Rev. B* **2010**, *82* (23), 235414.

(2) Dai, Z.; Liu, L.; Zhang, Z. Strain Engineering of 2D Materials: Issues and Opportunities at the Interface. *Adv. Mater.* **2019**, *31* (45), 1805417.

(3) Torelli, D.; Olsen, T. Calculating Critical Temperatures for Ferromagnetic Order in Two-Dimensional Materials. *2D Mater.* **2018**, *6* (1), 015028.

(4) Xu, C.; Feng, J.; Xiang, H.; Bellaiche, L. Interplay between Kitaev Interaction and Single Ion Anisotropy in Ferromagnetic $CrI_3$ and $CrGeTe_3$ Monolayers. *Npj Comput. Mater.* **2018**, *4* (1), 57.

(5) Huang, C.; Feng, J.; Wu, F.; Ahmed, D.; Huang, B.; Xiang, H.; Deng, K.; Kan, E. Toward Intrinsic Room-Temperature Ferromagnetism in Two-Dimensional Semiconductors. *J. Am. Chem. Soc.* **2018**, *140* (36), 11519–11525.

(6) Sivadas, N.; Daniels, M. W.; Swendsen, R. H.; Okamoto, S.; Xiao, D. Magnetic Ground State of Semiconducting Transition-Metal Trichalcogenide Monolayers. *Phys. Rev. B* **2015**, *91* (23), 235425.

(7) Binder, K. *Monte Carlo Methods in Statistical Physics*; Springer Science & Business Media, 2012.

(8) McGuire, M. A.; Dixit, H.; Cooper, V. R.; Sales, B. C. Coupling of Crystal Structure and Magnetism in the Layered, Ferromagnetic Insulator $CrI_3$. *Chem. Mater.* **2015**, *27* (2), 612–620.

(9) Webster, L.; Yan, J.-A. Strain-Tunable Magnetic Anisotropy in Monolayer $CrCl_3$, $CrBr_3$, and $CrI_3$. *Phys. Rev. B* **2018**, *98* (14), 144411.

(10) Zhang, W.-B.; Qu, Q.; Zhu, P.; Lam, C.-H. Robust Intrinsic Ferromagnetism and Half Semiconductivity in Stable Two-Dimensional Single-Layer Chromium Trihalides. *J. Mater. Chem. C* **2015**, *3* (48), 12457–12468.

(11) Huang, B.; Clark, G.; Navarro-Moratalla, E.; Klein, D. R.; Cheng, R.; Seyler, K. L.; Zhong, D.; Schmidgall, E.; McGuire, M. A.; Cobden, D. H.; et al. Layer-Dependent Ferromagnetism in a van Der Waals Crystal down to the Monolayer Limit. *Nature* **2017**, *546* (7657), 270–273.

(12) Lin, G. T.; Zhuang, H. L.; Luo, X.; Liu, B. J.; Chen, F. C.; Yan, J.; Sun, Y.; Zhou, J.; Lu, W. J.; Tong, P.; et al. Tricritical Behavior of the Two-Dimensional Intrinsically Ferromagnetic Semiconductor $CrGeTe_3$. *Phys. Rev. B* **2017**, *95* (24), 245212.

(13) Lin, M.-W.; Zhuang, H. L.; Yan, J.; Ward, T. Z.; Puretzky, A. A.; Rouleau, C. M.; Gai, Z.; Liang, L.; Meunier, V.; Sumpter, B. G.; et al. Ultrathin Nanosheets of $CrSiTe_3$: A Semiconducting Two-Dimensional Ferromagnetic Material. *J. Mater. Chem. C* **2016**, *4* (2), 315–322.

(14) Kong, T.; Stolze, K.; Timmons, E. I.; Tao, J.; Ni, D.; Guo, S.; Yang, Z.; Prozorov, R.; Cava, R. J. $VI_3$ —a New Layered Ferromagnetic Semiconductor. *Adv. Mater.* **2019**, *31* (17), 1808074.

(15) Son, S.; Coak, M. J.; Lee, N.; Kim, J.; Kim, T. Y.; Hamidov, H.; Cho, H.; Liu, C.; Jarvis, D. M.; Brown, P. A. C.; et al. Bulk Properties of the van Der Waals Hard Ferromagnet $VI_3$. *Phys. Rev. B* **2019**, *99* (4), 041402.

(16) Tian, S.; Zhang, J.-F.; Li, C.; Ying, T.; Li, S.; Zhang, X.; Liu, K.; Lei, H. Ferromagnetic van Der Waals Crystal $VI_3$. *J. Am. Chem. Soc.* **2019**, *141* (13), 5326–5333.
